# Supplementary material for: Electrostatic Correlation Augmented Self-Consistent Field Theory and Its Application to Polyelectrolyte Brushes
Source: arXiv:2404.09103 source file (2024-06-28)
Supplement: Supplementary file 1 [file SI.pdf]

# Supplementary Material for

## Ion Correlation Induced Non-monotonic Height Change and Microphase Separation of Polyelectrolyte Brushes

Chao Duan[1], Nikhil R. Agrawal[1], and Rui Wang[1,2,*]

1. Department of Chemical and Biomolecular Engineering, University of California Berkeley, CA 94720, USA

2. Materials Sciences Division, Lawrence Berkeley National Lab, Berkeley, California 94720, USA

* correspondence to: ruiwang325@berkeley.edu

## I. Derivation of the Electrostatic Fluctuation Augmented Self-Consistent Field Theory

In this section, we provide the detailed derivation of the electrostatic fluctuation augmented self-consistent field theory. The general formulation for polyelectrolyte (PE) solutions is in given **Sec. 1.1**. The specification of the theory to PE brushes in salt solutions is provided in **Sec. 1.2**.

### 1.1. General theory for PE solutions

We consider a general system consisting of $n_P$ negatively charged PEs each with $N_P$ monomers in an electrolyte solution which contains $n_S$ solvent molecules, $n_C$ monovalent counterions ($z_C = +1$) and $n_\pm$ salt ions with valency $z_\pm$. To more accurately describe the charge interactions, the ionic charge is modeled by a finite spread function $h_K(\mathbf{r}, \mathbf{r}')$ ($K = P, C, \pm$) instead of using the point-charge model[1, 2]. For convenience, we take $h_K(\mathbf{r}, \mathbf{r}')$ to be Gaussian which retains the Born radius $a_K$. The smeared charge model for PE widely used in existing theories fails to capture any correlations between charged monomers as well as between them and mobile ions. We adopt a discrete Gaussian chain model where each monomer is a charged particle with valency $z_P$. The number of dissociated counterions is thus $n_C = -z_P n_P N_P$.

The grand canonical partition function can be written as

$$\mathcal{Z} = \sum_{n_P=0}^{\infty} \frac{e^{\mu_P n_P}}{n_P! v_P^{N_P n_P}} \prod_{l=1}^{n_P} \int \hat{D}\{\mathbf{R}_l\} \prod_{\gamma=S,C,\pm} \sum_{n_\gamma=0}^{\infty} \frac{e^{\mu_\gamma n_\gamma}}{n_\gamma! v_\gamma^{n_\gamma}} \prod_{m=1}^{n_\gamma} \int d\mathbf{r}_{\gamma,m} \exp\left(-H\right) \prod_{\mathbf{r}} \delta\left[\sum_{K=P,S,C,\pm} v_K \hat{\rho}_K(\mathbf{r}) - 1\right] \tag{S1}$$

where $v_P$ and $v_\gamma$ are the volume of the PE segments and small molecules, respectively. For simplicity, we assume $v_P = v_S = v$. $\mu_K$ ($K = P, S, C, \pm$) is the chemical potential of PE, solvent, counterion and salt ions, respectively. $\int \hat{D}\{\mathbf{R}_l\} = \int D\{\mathbf{R}_l\}$ denotes integration over all chain configurations weighted by the statistics of connecting bonds with a transition probability $\Phi(\mathbf{R})$ [3]. $\hat{\rho}_K(\mathbf{r})$ are the local instantaneous number density of species $K$. The $\delta$ functional accounts for the incompressibility. The Hamiltonian $H$ in Eq. S1 is given by

$$H = \chi v \int d\mathbf{r} \hat{\rho}_P(\mathbf{r}) \hat{\rho}_S(\mathbf{r}) + \frac{1}{2} \int d\mathbf{r} d\mathbf{r}' \hat{\rho}_e(\mathbf{r}) C(\mathbf{r}, \mathbf{r}') \hat{\rho}_e(\mathbf{r}') \tag{S2}$$

where $\hat{\rho}_e(\mathbf{r}) = \sum_{K=P,C,\pm} z_K h_K * \hat{\rho}_K(\mathbf{r})$ is the net charge density. We use the short-hand notation $h * A(\mathbf{r}) = \int d\mathbf{r}' h(\mathbf{r} - \mathbf{r}') A(\mathbf{r}')$ to represent the local spatial averaging of quantity $A(\mathbf{r})$ by the charge distribution function $h(\mathbf{r} - \mathbf{r}')$ [1, 2]. $C(\mathbf{r}, \mathbf{r}')$ is the Coulomb operator

$$-\nabla \cdot [\epsilon(\mathbf{r}) \nabla C(\mathbf{r}, \mathbf{r}')] = \delta(\mathbf{r} - \mathbf{r}') \tag{S3}$$

The transfer from particle-based to field-based representation is achieved through the identity transformation as:

$$1=\int D\rho_K\prod_{\mathbf{r}}\delta[\rho_K(\mathbf{r})-\hat{\rho}_K(\mathbf{r})]=\int D\rho_K DW_K\exp\left\{i\int d\mathbf{r}W_K(\mathbf{r})[\rho_K(\mathbf{r})-\hat{\rho}_K(\mathbf{r})]\right\}\quad(K=P,S,C,\pm)\tag{S4}$$

where the right hand side of the equation arises from the Fourier representation of the $\delta$-function with $W_K(\mathbf{r})$ being the Fourier conjugate field to $\rho_K(\mathbf{r})$. To further decouple the interactions between charged particles, Hubbard-Stratonovich transform is performed for $\hat{\rho}_e(\mathbf{r})$, which introduces the conjugate field $\Psi(\mathbf{r})$

$$\exp\left\{-\frac{\beta e^2}{2}\int d\mathbf{r}d\mathbf{r}'\hat{\rho}_e(\mathbf{r})C(\mathbf{r},\mathbf{r}')\hat{\rho}_e(\mathbf{r}')\right\}=\mathcal{N}_C\int D\Psi\exp\left\{-\frac{\beta}{2}\int d\mathbf{r}d\mathbf{r}'\Psi(\mathbf{r})C^{-1}(\mathbf{r},\mathbf{r}')\Psi(\mathbf{r}')-i\int d\mathbf{r}\hat{\rho}_e(\mathbf{r})\beta e\Psi(\mathbf{r})\right\}\tag{S5}$$

Where $\mathcal{N}_C^{-1}=\int D\Psi\exp\{-(\beta/2)\int d\mathbf{r}d\mathbf{r}'\Psi(\mathbf{r})C^{-1}(\mathbf{r},\mathbf{r}')\Psi(\mathbf{r}')\}$ is the normalization constant. To economize notation, we rescale $\Psi(\mathbf{r})$ by $1/(\beta e)$ and rescale $\epsilon(\mathbf{r})$ by $\beta e^2$. Eq. S5 can then be rewritten as:

$$\exp\left[-\frac{\beta}{2}\int d\mathbf{r}d\mathbf{r}'\hat{\rho}_e(\mathbf{r})C(\mathbf{r},\mathbf{r}')\hat{\rho}_e(\mathbf{r}')\right]=\mathcal{N}_C\int D\Psi\exp\left\{\int d\mathbf{r}\left[\frac{1}{2}\nabla\cdot[\epsilon(\mathbf{r})\nabla\Psi(\mathbf{r})]-\sum_{K=P,C,\pm}z_K h_K*\hat{\rho}_K(\mathbf{r})i\Psi(\mathbf{r})\right]\right\}\tag{S6}$$

The partition function $\mathcal{Z}$ in Eq. S1 can then be cast into the following functional integral

$$\begin{aligned}\mathcal{Z}=&\mathcal{N}_C\int D\rho_P D\rho_S DW_P DW_S D\Psi D\Xi\sum_{n_P=0}^{\infty}\frac{e^{\mu_P n_P}}{n_P!v_P^{N_P n_P}}\prod_{l=1}^{n_P}\int D\{\mathbf{R}^l\}\prod_{\gamma=S,C,\pm}\sum_{n_\gamma=0}^{\infty}\frac{e^{\mu_\gamma n_\gamma}}{n_\gamma!v_\gamma^{n_\gamma}}\prod_{m=1}^{n_\gamma}\int d\mathbf{r}_{\gamma,m}\\&\cdot\exp\left\{\int d\mathbf{r}\left[-\sum_{l=1}^{n_P}\sum_{i=1}^{N_P-1}\Phi(\mathbf{R}_{l,i+1}-\mathbf{R}_{l,i})-\chi v\rho_P\rho_S+iW_P(\rho_P-\hat{\rho}_P)+iW_S(\rho_S-\hat{\rho}_S)+\frac{i\Xi}{v}\left(\sum_{K=P,S,C,\pm}v_K\rho_K-1\right)\right]\right\}\\&\cdot\exp\left\{\int d\mathbf{r}\left[\frac{1}{2}\Psi(\mathbf{r})\nabla\cdot[\epsilon(\mathbf{r})\nabla\Psi(\mathbf{r})]-\sum_{K=P,C,\pm}z_K h_K*\hat{\rho}_K(\mathbf{r})i\Psi(\mathbf{r})\right]\right\}\end{aligned}\tag{S7}$$

Note that we assume $v_P=v_S=v$ and insert the Fourier representation of the incompressibility condition

$$\prod_{\mathbf{r}}\delta\left[\sum_{K=P,S,C,\pm}v_K\rho_K(\mathbf{r})-1\right]=\int D\Xi\exp\left\{i\int d\mathbf{r}\Xi(\mathbf{r})\left[\sum_{K=P,S,C,\pm}v_K\rho_K(\mathbf{r})-1\right]\right\}$$

Then Eq. S7 can be rewritten as $\mathcal{Z}=\int D\rho_P D\rho_S DW_P DW_S D\Psi D\Xi\exp\{-\mathcal{L}[\rho_P,\rho_S,W_P,W_S,\Psi,\Xi]\}$ with the action $\mathcal{L}$:

$$\begin{aligned}\mathcal{L}[\rho_P,\rho_S,W_P,W_S,\Psi,\Xi]=&\lambda_P Q_P+\lambda_S Q_S+\int d\mathbf{r}\left[-\chi v\rho_P\rho_S+iW_P\rho_P+iW_S\rho_S+i\Xi\left(\rho_P+\rho_S-v^{-1}\right)\right]\\&+\int d\mathbf{r}\left[\frac{1}{2}\Psi\nabla\cdot(\epsilon\nabla\Psi)+\sum_{K=C,\pm}\lambda_K e^{-iz_K h_K*\Psi(\mathbf{r})-iv_K\Xi(\mathbf{r})/v}\right]+\ln\mathcal{N}_C\end{aligned}\tag{S8}$$

where $\lambda_P=e^{\mu_P}/v_P^{N_P}$ is the fugacity of PE, and $\lambda_K=e^{\mu_K}/v_K$ is the fugacity of the small molecule $K$ ($K=S,C,\pm$). $Q_S=\int d\mathbf{r}e^{-iW_S(\mathbf{r})}$ is the partition function of solvents, and $Q_P=\int D\mathbf{R}\exp[-\sum_{i=1}^{N_P-1}\Phi(\mathbf{R}_{i+1}-\mathbf{R}_i)-\sum_{i=1}^{N_P}iW_P(\mathbf{R}_i)-\sum_{i=1}^{N_P}iz_P h_P*\Psi(\mathbf{R}_i)]$ is the single-chain partition function of PE.

To account for the electrostatic fluctuation, the Gibbs-Feynman-Bogoliubov variational approach is used to estimate the integral in $\Psi$ for calculating the grand free energy $\mathcal{F}$ [1, 2]. We take the reference action to be of the Gaussian form centered around the mean potential, $-i\psi$

$$\mathcal{F}=-\ln\mathcal{Z}\approx-\ln\mathcal{Z}_{ref}+\langle\mathcal{L}[\rho_P,\rho_S,W_P,W_S,\Psi,\Xi]-\mathcal{L}_{ref}[\Psi,\psi,G]\rangle_{\mathcal{L}_{ref}}\tag{S9}$$

$$\mathcal{L}_{ref}[\Psi,\psi,G]=\frac{1}{2}\int d\mathbf{r}d\mathbf{r}'[\Psi(\mathbf{r})+i\psi(\mathbf{r})]G(\mathbf{r},\mathbf{r}')[\Psi(\mathbf{r}')+i\psi(\mathbf{r}')] \tag{S10}$$

where the short-hand notation $\langle\cdots\rangle_{\mathcal{A}}$ is an average taken in the reference ensemble with action $\mathcal{A}$. We use the above Gaussian reference action to perform the variation of $\mathcal{Z}$ with respect to the mean electrostatic potential $\psi$ and Green function $G$ [1, 2]. For other fields $\rho_P$, $\rho_S$, $W_P$, $W_S$, and $\Xi$, we take the saddle-point approximation ($\rho_P$, $\rho_S$, $-i\omega_P$, $-i\omega_S$, and $-i\xi$) [3]. The variational free energy yields:

$$\begin{aligned}\mathcal{F}_{var}=&-\lambda_PQ_P-\lambda_SQ_S+\int d\mathbf{r}\Big\{\chi v\rho_P\rho_S-\omega_P\rho_P-\omega_S\rho_S-\xi\left(\rho_P+\rho_S-v^{-1}\right)+\frac{1}{2}\psi(\mathbf{r})\nabla\cdot[\epsilon(\mathbf{r})\nabla\psi(\mathbf{r})]\\&-\sum_{K=C,\pm}\lambda_Ke^{-z_K\psi(\mathbf{r})-u_K^0(\mathbf{r})-v_K\xi(\mathbf{r})/v}\Big\}+\frac{1}{2}\int d\mathbf{r}d\mathbf{r}'[C^{-1}(\mathbf{r},\mathbf{r}')-G^{-1}(\mathbf{r},\mathbf{r}')]G(\mathbf{r},\mathbf{r}')-\frac{1}{2}\ln\left(\frac{\det G}{\det C}\right)\end{aligned} \tag{S11}$$

$$u_K^0(\mathbf{r})=\frac{z_K^2}{2}\int d\mathbf{r}'d\mathbf{r}''h_K(\mathbf{r}-\mathbf{r}')G(\mathbf{r}',\mathbf{r}'')h_K(\mathbf{r}''-\mathbf{r}) \tag{S12}$$

where $u_K^0$ is the self energy of ions individually evaluated from their own charge spread. The partition function of solvents becomes $Q_S=\int d\mathbf{r}e^{-\omega_S(\mathbf{r})}$. The single-chain partition function of PE becomes

$$\begin{aligned}Q_P=&\int D\mathbf{R}\exp\left[-\sum_{i=1}^{N_P-1}\Phi(\mathbf{R}_{i+1}-\mathbf{R}_i)-\sum_{i=1}^{N_P}\omega_P(\mathbf{R}_i)-\sum_{i=1}^{N_P}z_P\psi(\mathbf{R}_i)\right]\\&\cdot\exp\left\{-\frac{z_P^2}{2}\int d\mathbf{r}'d\mathbf{r}''\left[\sum_{i=1}^{N_P}h_P(\mathbf{R}_i-\mathbf{r}')\right]G(\mathbf{r}',\mathbf{r}'')\left[\sum_{j=1}^{N_P}h_P(\mathbf{r}''-\mathbf{R}_j)\right]\right\}\end{aligned} \tag{S13}$$

where the exponent of the term in the second line is the electrostatic self-energy of the entire PE chain. It is clear that this self-energy is coupled to the chain conformation $\mathbf{R}$, which for each monomer $i$ contains the individual contribution $u_P^0(\mathbf{R}_i)$ and an extra contribution from all other intra-chain monomers $u_P^{ex}(\mathbf{R}_i;i)=(z_P^2/2)\int d\mathbf{r}'d\mathbf{r}''h_P(\mathbf{R}_i-\mathbf{r}')G(\mathbf{r}',\mathbf{r}'')[\sum_{j\neq i}^{N_P}h_P(\mathbf{r}''-\mathbf{R}_j)]$. Conventional evaluation of $Q_P$ requires replacing the direct calculation of the complicated functional integral by solving the partial differential equations of propagators [3], which however is difficult to realize due to the 2-body interaction term $u_P^{ex}$ contained in the self-energy of PE. To circumvent this difficulty, we approximate $Q_P$ by evaluating the 2-body contributions $H^{ex}[\mathbf{R}_i,\mathbf{R}_j]$

$$H^{ex}[\mathbf{R}_i,\mathbf{R}_j]=\sum_{i=1}^{N_P}u_P^{ex}(\mathbf{R}_i;i)=\sum_{i=1}^{N_P}\sum_{j\neq i}^{N_P}\frac{z_P^2}{2}\int d\mathbf{r}'d\mathbf{r}''h_P(\mathbf{R}_i-\mathbf{r}')G(\mathbf{r}',\mathbf{r}'')h_P(\mathbf{r}''-\mathbf{R}_j) \tag{S14}$$

via an averaging under the reference ensemble with 1-body Hamiltonian $H^0[\mathbf{R}_i]$

$$H^0[\mathbf{R}_i]=\sum_{i=1}^{N_P-1}\Phi(\mathbf{R}_{i+1}-\mathbf{R}_i)+\sum_{i=1}^{N_P}[\omega_P(\mathbf{R}_i)+z_P\psi(\mathbf{R}_i)+u_P^0(\mathbf{R}_i)] \tag{S15}$$

The the procedure of the average is as follows:

$$Q_P=\int D\mathbf{R}e^{-H^0[\mathbf{R}_i]-H^{ex}[\mathbf{R}_i,\mathbf{R}_j]}=Q_0\langle e^{-H^{ex}[\mathbf{R}_i,\mathbf{R}_j]}\rangle_{H^0} \tag{S16}$$

with $Q_0=\int D\mathbf{R}e^{-H^0[\mathbf{R}_i]}$. To evaluate a 2-body Hamiltonian in a one-body reference in the second equality in Eq. S16, we first fix the position of the $i$-th monomer $\mathbf{R}_i$ and calculate the average with respect to the position of the $j$-th monomer $\mathbf{R}_j$ to obtain $\langle e^{-H^{ex}[\mathbf{R}_i,\overline{\mathbf{R}_j}]}\rangle_{H^0}$. We then take the average with respect to $\mathbf{R}_i$ as:

$$Q_P=\int D\mathbf{R}e^{-H^0[\mathbf{R}_i]}\langle e^{-H^{ex}[\mathbf{R}_i,\overline{\mathbf{R}_j}]}\rangle_{H^0}\approx\int D\mathbf{R}e^{-H^0[\mathbf{R}_i]-\langle H^{ex}[\mathbf{R}_i,\overline{\mathbf{R}_j}]\rangle_{H^0}} \tag{S17}$$

where the second equality assumes that $2n$-body correlations ($n \geq 2$) are neglected. Then $Q_P$ can be evaluated via the forward (backward) chain propagators $q(\mathbf{r}; i)$ ($q^\dagger(\mathbf{r}; i)$)

$$Q_P = \int d\mathbf{r} q(\mathbf{r}; i) e^{V_P(\mathbf{r}; i)} q^\dagger(\mathbf{r}; i) \tag{S18}$$

$$q(\mathbf{r}; i) = e^{-V_P(\mathbf{r}; i)} \int d\mathbf{r}' \Phi(\mathbf{r} - \mathbf{r}') q(\mathbf{r}'; i-1) \tag{S19a}$$

$$q^\dagger(\mathbf{r}; i) = e^{-V_P(\mathbf{r}; i)} \int d\mathbf{r}' \Phi(\mathbf{r} - \mathbf{r}') q^\dagger(\mathbf{r}'; i+1) \tag{S19b}$$

where the total interaction field experienced by the $i$-th monomer $V_P(\mathbf{r}; i) = V_P^0(\mathbf{r}) + u_P^{ex}(\mathbf{r}; i)$ with $V_P^0(\mathbf{r}) = \omega_P(\mathbf{r}) + z_P\psi(\mathbf{r}) + u_P^0(\mathbf{r})$. The extra self-energy $u_P^{ex}(\mathbf{r}; i)$ experienced by PE monomer becomes

$$u_P^{ex}(\mathbf{r}; i) = \frac{z_P^2}{2} \left[ \sum_{j=i+1}^{N_P} \frac{\int d\mathbf{r}' g_0(\mathbf{r}, \mathbf{r}'; i, j) G(\mathbf{r}, \mathbf{r}') e^{V_P^0(\mathbf{r}')} q_0^\dagger(\mathbf{r}'; j)}{q_0^\dagger(\mathbf{r}; i)} + \sum_{j=1}^{i-1} \frac{\int d\mathbf{r}' q_0(\mathbf{r}'; j) e^{V_P^0(\mathbf{r}')} G(\mathbf{r}', \mathbf{r}) g_0^\dagger(\mathbf{r}', \mathbf{r}; j, i)}{q_0(\mathbf{r}; i)} \right] \tag{S20}$$

where the chain propagator $q_0(\mathbf{r}; j)$ ($q_0^\dagger(\mathbf{r}; j)$) and intra-chain correlation function $g_0(\mathbf{r}, \mathbf{r}'; i, j)$ ($g_0(\mathbf{r}', \mathbf{r}; j, i)$) are subject to the same recurrence relation (Eq. S19) as $q(\mathbf{r}; j)$ ($q^\dagger(\mathbf{r}; j)$) but with interaction field $V_P^0$ corresponding to the reference state. The mean electrostatic potential $\psi$ is determined by $\delta\mathcal{F}_{var}/\delta\psi = 0$, leading to the Poisson equation:

$$-\nabla \cdot [\epsilon(\mathbf{r}) \nabla \psi(\mathbf{r})] = \sum_{K=P,C,\pm} z_K \rho_K(\mathbf{r}) \tag{S21}$$

with $\rho_K(\mathbf{r})$ ($K = C, \pm$) the number density of mobile ions:

$$\rho_K(\mathbf{r}) = \lambda_K e^{-z_K\psi(\mathbf{r}) - u_K^0(\mathbf{r}) - v_K\xi(\mathbf{r})/v} \quad (K = C, \pm) \tag{S22}$$

The Green function is determined by $\delta\mathcal{F}_{var}/\delta G = 0$, leading to

$$-\nabla_\mathbf{r} \cdot [\epsilon(\mathbf{r}) \nabla_\mathbf{r} G(\mathbf{r}, \mathbf{r}')] + 2I_0(\mathbf{r}) G(\mathbf{r}, \mathbf{r}') + \int d\mathbf{r}'' 2I_{ex}(\mathbf{r}, \mathbf{r}'') G(\mathbf{r}'', \mathbf{r}') = \delta(\mathbf{r} - \mathbf{r}') \tag{S23}$$

where $I_0(\mathbf{r}) = \sum_{K=P,C,\pm} z_K^2 \rho_K(\mathbf{r})/2$ is the local component of ionic strength. Different from the commonly used Green function, the ionic strength of PE systems has an extra non-local contribution $I_{ex}(\mathbf{r}, \mathbf{r}')$ from the long-range charge spread of polymer

$$\begin{aligned} I_{ex}(\mathbf{r}, \mathbf{r}') = \frac{z_P^2}{2} \sum_{i=1}^{N_P} \lambda_P e^{V_P(\mathbf{r}; i)} \Bigg[ & \sum_{j=i+1}^{N_P} q(\mathbf{r}; i) g(\mathbf{r}, \mathbf{r}'; i, j) G(\mathbf{r}, \mathbf{r}') e^{V_P(\mathbf{r}'; j)} q^\dagger(\mathbf{r}'; j) \\ & + \sum_{j=1}^{i-1} q(\mathbf{r}'; j) e^{V_P(\mathbf{r}'; j)} G(\mathbf{r}', \mathbf{r}) g^\dagger(\mathbf{r}', \mathbf{r}; j, i) q^\dagger(\mathbf{r}; i) \Bigg] \end{aligned} \tag{S24}$$

Taking the Saddle-point approximation for number density of PE and solvents $\rho_P$, $\rho_S$, conjugate fields $\omega_P$, $\omega_S$, as well as incompressibility field $\xi$, we obtain

$$\omega_P(\mathbf{r}) = \chi v \rho_S(\mathbf{r}) - \xi(\mathbf{r}) - \frac{1}{2} \frac{\partial \epsilon(\mathbf{r})}{\partial \rho_P(\mathbf{r})} [\nabla \psi(\mathbf{r})]^2 \tag{S25a}$$

$$\omega_S(\mathbf{r}) = \chi v \rho_P(\mathbf{r}) - \xi(\mathbf{r}) - \frac{1}{2} \frac{\partial \epsilon(\mathbf{r})}{\partial \rho_S(\mathbf{r})} [\nabla \psi(\mathbf{r})]^2 \tag{S25b}$$

$$\rho_P(\mathbf{r}) = \lambda_P \sum_{i=1}^{N_P} q(\mathbf{r};i) e^{V_P(\mathbf{r};i)} q^\dagger(\mathbf{r};i) \tag{S25c}$$

$$\rho_S(\mathbf{r}) = \lambda_S e^{-\omega_S(\mathbf{r})} \tag{S25d}$$

$$0 = \sum_{K=P,S,C,\pm} v_K \rho_K(\mathbf{r}) - 1 \tag{S25e}$$

For the system consisting of $n_P$ PE chains immersed in a salt solutions in contact with a bulk salt solution with given chemical potentials of salt ions and solvent molecules, $\mu_\pm$ and $\mu_S$, respectively, $\lambda_\pm = e^{\mu_\pm}/v_\pm$ and $\lambda_S = e^{\mu_S}/v$. $\mu_\pm$ and $\mu_S$ are determined from the bulk salt concentration $\rho_b$. The fugacity of PE $\lambda_P = e^{\mu_P}/v$ and counterion $\lambda_C = e^{\mu_C}/v_C$ are determined from the normalization condition: $\lambda_P = n_P/Q_P$ and $\lambda_C = n_C/Q_C$ with $Q_C = \int d\mathbf{r} e^{-z_C\psi(\mathbf{r}) - u_C^0(\mathbf{r}) - v_C\xi(\mathbf{r})/v}$. The resulting free energy of the semi-canonical ensemble (with the fixed number of PEs and counterions) is thus:

$$F = -n_P \ln Q_P - n_C \ln Q_C - \lambda_S Q_S + \int d\mathbf{r} \Big\{ \chi v \rho_P \rho_S - \omega_P \rho_P - \omega_S \rho_S - \xi\left(\rho_P + \rho_S - v^{-1}\right) + \frac{1}{2}\psi(\mathbf{r}) \nabla \cdot [\epsilon(\mathbf{r}) \nabla \psi(\mathbf{r})] \\ - \sum_{K=\pm} \lambda_K e^{-z_K\psi(\mathbf{r}) - u_K^0(\mathbf{r}) - v_K\xi(\mathbf{r})/v} \Big\} + \frac{1}{2}\int d\mathbf{r} d\mathbf{r}' [C^{-1}(\mathbf{r},\mathbf{r}') - G^{-1}(\mathbf{r},\mathbf{r}')] G(\mathbf{r},\mathbf{r}') - \frac{1}{2}\ln\left(\frac{\det G}{\det C}\right) \tag{S26}$$

The last two terms in the free energy Eq. S26 represent the contributions arising from the electrostatic correlation [1, 2], which can be evaluated by the "charging method" [2].

### 1.2. Application to a specific system of PE brushes

We consider a planar surface which is uniformly grafted by $n_P$ PEs. The grafting density $\sigma = n_P/A$ where $A$ is the area of the surface. Since each chain is tethered on the surface, the partition function in Eq. S1 need to be modified as:

$$\mathcal{Z} = \sum_{n_P=0}^{\infty} \frac{e^{\mu_P n_P}}{n_P! v_P^{N_P n_P}} \prod_{l=1}^{n_P} \int \hat{D}\{\mathbf{R}_l\} \prod_{\gamma=S,C,\pm} \sum_{n_\gamma=0}^{\infty} \frac{e^{\mu_\gamma n_\gamma}}{n_\gamma! v_\gamma^{n_\gamma}} \prod_{m=1}^{n_\gamma} \int d\mathbf{r}_{\gamma,m} \exp(-H) \\ \cdot \prod_{\mathbf{r}} \delta\left[\sum_{K=P,S,C,\pm} v_K \hat{\rho}_K(\mathbf{r}) - 1\right] \prod_{l=1}^{n_P} \delta\left(\mathbf{R}_{l,1} - \mathbf{r}_l\right) \tag{S27}$$

where the same Hamiltonian in Eq. S2 is adopted. The last $\delta$-functions reinforce the constraint that the position of the first monomer $\mathbf{R}_{l,1}$ of the $l$-th PE chain is fixed at $\mathbf{r}_l = (x_l, y_l, z_l)$ with $z_l = 0$ for the plate surface. Due to this tethering effect, the polymer density now reads:

$$\rho_P(\mathbf{r}) = \sum_{i=1}^{N_P} \tilde{q}(\mathbf{r};i) e^{V_P(\mathbf{r};i)} q^\dagger(\mathbf{r};i) \tag{S28}$$

Note that the forward propagator $\tilde{q}(\mathbf{r};i)$ starts from the grafting plate of all grafted PE chains, which satisfies the same equation as Eq. S19a; however, the initial condition becomes $\tilde{q}(\mathbf{r};1) = \sum_{l=1}^{n_P} \delta(\mathbf{r} - \mathbf{r}_l)/q^\dagger(\mathbf{r}_l;1)$ [3].The backward propagator $q^\dagger(\mathbf{r};i)$ satisfies the same equation as Eq. S19b with the initial condition $q^\dagger(\mathbf{r};N) = e^{-V_P(\mathbf{r};N)}$ because the chain end not tethered to the surface is free.

Because each polymer is now tethered at different positions, they need to be treated separately. The single-chain partition function in Eq. S18 also needs to be modified. We now define $\tilde{Q}_P$ as the partition function of all polymers

as:

$$\ln\tilde{Q}_P = \sum_{l=1}^{n_P} \ln q^\dagger(\mathbf{r}_l; 1) \tag{S29}$$

If the grafting density $\sigma$ is large enough, we can replace the sum over chains in Eq. S29 by a quenched average over the locations of the tethering points such that $\ln\tilde{Q}_P = \sigma \int dxdy \ln q^\dagger(x, y, 0; 1)$ [3]. Similarly, $\tilde{q}(\mathbf{r}; 1) = \sigma\delta(z)/q^\dagger(\mathbf{r}; 1)$. The free energy of the PE brush system is:

$$F = -\ln\tilde{Q}_P - n_C \ln Q_C - \lambda_S Q_S + \int d\mathbf{r} \Big\{ \chi v \rho_P \rho_S - \omega_P \rho_P - \omega_S \rho_S - \xi \left(\rho_P + \rho_S - v^{-1}\right) + \frac{1}{2}\psi(\mathbf{r})\nabla \cdot [\epsilon(\mathbf{r})\nabla\psi(\mathbf{r})]$$
$$- \sum_{K=\pm} \lambda_K e^{-z_K\psi(\mathbf{r}) - u_K^0(\mathbf{r}) - v_K\xi(\mathbf{r})/v} \Big\} + \frac{1}{2}\int d\mathbf{r} d\mathbf{r}' [C^{-1}(\mathbf{r}, \mathbf{r}') - G^{-1}(\mathbf{r}, \mathbf{r}')] G(\mathbf{r}, \mathbf{r}') - \frac{1}{2}\ln\left(\frac{\det G}{\det C}\right) \tag{S30}$$

## II. Details of Numerical Calculations

In this section, numerical details of solving the key equations are provided. The equilibrium structure and the free energy can be obtained by solving Eqs. S12, S18-S25 iteratively until convergence. Both chain propagators (Eq. S19) and Poisson equation (Eq. S21) can be solved by fast Fourier transform using the FFTW package [4]. The Green function $G(\mathbf{r}, \mathbf{r}')$ (Eq. S23) can be solved by using the alternating-direction implicit method(ADI) [5]. The efficiency of solving $G$ can be improved by decompositing it into a short- and a long-range parts, i. e. $G = G_s + G_l$ [2]. The short-range part $G_s$ accounting for the local electrostatic environment can be analytically tractable [2]. The long-range part $G_l$ takes care of spatially varying ionic strength and dielectric permittivity. For three dimensional real space, numerically solving $G_l$ is still computationally challenging (due to the six dimensions in the numerical calculation). Fortunately, this challenge can be solved by considering the fact that $G_l$ captures the electrostatic effects that act at a much larger length scale than the ion size. Hence, during the iteration, the relative change of $G_l$ should be much smaller than $G_s$, which enables us to update $G_l$ every $m_G$ ($m_G \gg 1$) iteration steps. Our calculations show that, for the systems focused in the current manuscript, $m_G = 500$ can be safely used to give the same final results. Taking together these improvements, the total computational cost involved in solving the Green function can be comparable to that of solving the chain propagators.

To further stabilize the convergence, we use the following strategy to update the fields. Fields conjugate to the density of polymer and solvent molecules are updated by a simple mixing rule, i. e., $\omega_{P,S}^{new} \leftarrow \lambda\omega_{P,S}^{new} + (1-\lambda)\omega_{P,S}^{old}$. The same rule is adopted for updating electrostatic potential $\psi$, self-energy $u_K$ ($K = P, C, \pm$), and Green function $G$. The field conjugated to the incompressibility condition is updated by $\xi^{new} \leftarrow \xi^{old} + \kappa(\sum_{K=P,S,\pm} v_K\rho_K - 1)$, where the second term on the r.h.s is adopted to reinforce the incompressibility.

## III. Derivation of the Scaling Equations

In this section, we provide detailed derivation of the analytical results of the scaling theory in the main text. Based on the previous efforts [6], we simplify the PE brush system into two homogeneous subsystems, i. e. the brush layer and the bulk salt solution. These two subsystems are in equilibrium if the conditions of both charge neutrality ($\sum_K z_K\rho_K = 0$) and force balance ($f_{\text{ela}} + f_{\text{int}} + f_{\text{ion}} = 0$) are satisfied. $f_{\text{ela}} \approx -\sigma h/Nb^2$ is the elastic stress due to chain deformation, where $h$ is the brush height, $\sigma$ is the grafting density. $f_{\text{int}} \approx w_2\rho_P^2 + w_3\rho_P^3$ is the non-electrostatic interaction between monomers. $\rho_P = \sigma N/h$ is the polymer density in the brush regime; $w_2$ and $w_3$ are the second and third virial coefficients, respectively. $f_{\text{ion}}$ is the electrostatic osmotic pressure including ion transnational entropy and ion correlation.

### 3.1. Effective relative charge on the brush $\Gamma$

In our new theory, the electrostatic correlation effect is captured by the self-energy of ions. For a homogeneous system, the self-energy of charge $K$ can be analytically expressed as

$$u_K = \frac{z_K^2}{8\pi\epsilon a_K} u(a_K\kappa) \tag{S31}$$

where $u$ is a universal function for all charge spread models. In particular, $u(x) = 1 - x\exp(x^2/\pi)\mathrm{erfc}(x/\sqrt{\pi})$ if the charge distribution function $h_K$ takes the Gaussian form [2]. For simplicity, all ions are set to have the same radius, $a_K = a$. Here we mainly focus on a higher salt concentration regime where ion screening or ion correlation effects become pronounced and the role of counterions can be neglected. It satisfies

$$\rho_b \gg \alpha\rho_P \tag{S32}$$

where $\alpha$ is the fraction of negatively charged monomers on the PE backbone and $\alpha = 1$ if PE is fully charged. For the $z_+ : 1$ salt solution adopted in the manuscript, using the Boltzmann distribution of the ion density (Eq. S22), we can eliminate the potential $\psi$ and obtain the following equations for relationship between the cation and anion density as:

$$\frac{\rho_+}{\rho_b}\left(\frac{\rho_-}{z_+\rho_b}\right)^{z_+} = \exp\left[-(u_+ - u_+^b) - z_+(u_- - u_-^b)\right] \tag{S33}$$

Note that the excluded volume of ions has been neglected ($v_C = v_\pm = 0$). We then define a $\delta\rho$ that satisfies $\delta\rho = \alpha\rho_P/z_+ - (\rho_+ - \rho_b)$, where $z_+\delta\rho$ can be understood as the effective charge remaining on the polymer after the adsorption of cations. $\delta\rho < 0$ indicates overcompensation of PE charges by cations. We have:

$$\rho_+ = \rho_b + \alpha\rho_P/z_+ - \delta\rho \tag{S34a}$$

$$\rho_- = z_+(\rho_b - \delta\rho) \tag{S34b}$$

where Eq. S34b comes from the charge neutrality condition. Under the assumption of $|\delta\rho| \ll \rho_b$, we can expand both the left hand side and the right hand side of Eq. S33 in terms of $\delta\rho$ and keep the first-order terms, which yields:

$$\delta\rho = \frac{\Gamma\alpha\rho_P}{z_+} \tag{S35}$$

where $\Gamma$ satisfies:

$$\frac{(z_+ + 1)\Gamma - 1}{\Gamma - 1} = -\frac{z_+(z_+ + 1)\kappa_b}{16\pi\epsilon}\frac{du}{d(a\kappa_b)} \tag{S36}$$

Based on Eq. S35, $\Gamma$ can be understood as the effective relative charge on the PE brushes after cation adsorption.

### 3.2. Electrostatic osmotic pressure $f_{\text{ion}}$

Using the "charging method" to evaluate the electrostatic correlation contribution in the free energy [2], the electrostatic osmotic pressure $f_{\text{ion}}$ including both the translational entropy of ions and the ion correlations can be expressed as

$$f_{\text{ion}} = \sum_{K=\pm}(\rho_K - \rho_K^b) - \left\{\sum_{K=P,\pm}\int_0^1 d\tau\rho_K\left[u_K(\tau) - u_K\right] - \sum_{K=\pm}\int_0^1 d\tau\rho_K^b\left[u_K^b(\tau) - u_K^b\right]\right\} \tag{S37}$$

where $0 \le \tau \le 1$ is the "charging" variable, and $u_K(\tau)$ is the self-energy corresponding to Green function solved under the ionic strength $\tau I_0$ [2]. Following a similar derivation using the expansion on Eq. S37 in terms of $\delta\rho$, we obtain

$$f_{\text{ion}} = \frac{\alpha^2\rho_P^2\Gamma}{z_+\rho_b} \tag{S38}$$

which indicates that the electrostatic osmotic pressure $f_{\text{ion}}$ is proportional to $\Gamma$. The sign of $f_{\text{ion}}$ is the same as the sign of $\Gamma$.

### 3.3. Scaling relationship of brush height in the four regimes

In the osmotic regime, effects of both ion screening and ion correlation is negligible. By balancing the attractive PE elastic stress with the repulsive counterion osmotic pressure [6], i. e. $f_{\text{ela}} + f_{\text{ion}} \approx 0$ with $f_{\text{ion}} \approx \rho_+ \approx \alpha\rho_P/z_+$ , we obtain the following scaling relationship

$$h \approx Nb\alpha^{1/2} \tag{S39a}$$

In the salted regime where the contribution from the tranlational entropy of ions is stronger than that of ion correlation, the net osmotic pressure keeps repulsive ($\Gamma > 0$ in Eq. S38) and PE brushes are still expanded. Using $f_{\text{ela}} + f_{\text{ion}} \approx 0$ with Eq. S38, the brush height can be obtained

$$h \approx Nb\alpha^{2/3}\left(\frac{\sigma\Gamma}{z_+ b}\right)^{1/3} \rho_b^{-1/3} \tag{S39b}$$

In the collapsed regime where the contribution from ion correlations is stronger than that of the translational entropy of ions, the net osmotic is attractive ($\Gamma < 0$ in Eq. S38) and PE brushes are collapsed. In such morphology, $f_{\text{ela}}$ can be neglected. The brush height is mainly determined by balancing the repulsive three-body interaction $f_{\text{int}} \approx w_3\rho_P^3$ and the attractive ion osmotic pressure, $f_{\text{int}} + f_{\text{ion}} \approx 0$, which yields

$$h \approx -Nb\alpha^{-2}\left(\frac{\sigma w_3 z_+}{\Gamma b}\right)\rho_b \tag{S39c}$$

In the neutral regime that salt concentration is high enough to completely neutralize the PE charges, the neutral brush behavior can be recovered. By balancing two-body interactions $f_{\text{int}} \approx w_2\rho_P^2$ and the elastic stress, i.e. $f_{\text{int}} + f_{\text{ela}} \approx 0$, the brush height can be obtained [6]

$$h \approx Nb\left(\frac{\sigma w_2}{b}\right)^{1/3} \tag{S39d}$$

### 3.4. Electrostatic potential $\psi$ in the brush region

Expanding the ion distribution in Eq. S22 in terms of $\delta\rho$ and inserting the relationship of Eq. S35, we can solve for the electrostatic potential $\psi$ in the brush region as:

$$\psi \approx -\frac{\alpha\rho_P}{z_+^2(z_+ + 1)}\left[(z_+^2 - 1)\Gamma + 1\right] \tag{S40}$$


[1] Z.-G. Wang, Phys. Rev. E **81**, 021501 (2010), URL `https://link.aps.org/doi/10.1103/PhysRevE.81.021501`.

[2] N. R. Agrawal and R. Wang, Phys. Rev. Lett. **129**, 228001 (2022), URL `https://link.aps.org/doi/10.1103/PhysRevLett.129.228001`.

[3] G. H. Fredrickson, *The Equilibrium Theory of Inhomogeneous Polymers*, International Series of Monographs on Physics (OUP Oxford, 2006), ISBN 9780198567295, URL `https://books.google.com/books?id=ZiwTDAAAQBAJ`.

[4] M. Frigo, *A Fast Fourier Transform Compiler*, Proceedings of the 1999 ACM SIGPLAN Conference on Programming Language Design and Implementation (PLDI '99) (Atlanta, Georgia, 1999).

[5] J. D. Hoffman and S. Frankel, *Numerical Methods for Engineers and Scientists* (CRC Press, 2018), ISBN 9781315274508, URL `http://dx.doi.org/10.1201/9781315274508`.

[6] E. B. Zhulina, T. M. Birshtein, and O. V. Borisov, Macromolecules **28**, 1491 (1995), ISSN 1520-5835, URL `http://dx.doi.org/10.1021/ma00109a021`.
